# Supplementary material for: Clustering RDF Databases Using Tunable-LSH
Source: arXiv:1504.02523 source file (2015-04-19)
Supplement: Supplementary file 1 [file appendix.tex]

\section{Additional Proofs}

Given a set of record utilization vectors $R = \{ \record{r_{1}}, \ldots, \record{r_{l}} \}$, where each vector has size $k$, 
let $R^{M} = \{ \record{P_{1}}, \ldots, \record{P_{l}} \}$ denote the coresponding set of points in the $k$-dimensional space with coordinates $\{ 0, 1 \}$ on each axis.
Furthermore, let $\delta( \cdot, \cdot )$ denote the edit distance between two record utilization vectors, and
let $\delta^{M}( \cdot, \cdot )$ denote the Manhattan distance between two points.
Then, for every $\record{r_{a}}, \record{r_{b}} \in R$,
$\delta( \record{r_{a}}, \record{r_{b}} ) = \delta^{M}( \record{P_{a}}, \record{P_{b}} )$,
where $ \record{P_{a}}, \record{P_{b}} \in R^{M} $ are the corresponding points for $\record{r_{a}}$ and $\record{r_{b}}$, respectively.

We prove Theorem ... by induction on the size of record utilization vectors ($k$).

\noindent \textbf{Base case:} 
We prove Theorem ... when $k=1$.
$\record{r_{i}}$ can be either $(0)$ or $(1)$, and so can $\record{r_{j}}$, hence, there are four cases to consider.
As shown in Fig ..., for all the four cases, edit distances are equal to the Manhattan distances.

\noindent \textbf{Inductive step:}
Assuming edit distances equal Manhattan distances for any pair of record utilization vectors with size $k \leq C$, we prove that the same statement holds for $k = C+1$.
First, note that for $k=C+1$, the Manhattan distance between (any) two points $P_{a}$ and $P_{b}$ is defined as:
\begin{align}
\delta^{M}( P_{a}, P_{b} ) = \sum\limits_{i=1}^{C+1} \abs{ P_{a}[i] - P_{b}[i] } \text{.}
\end{align}
Therefore, going from $k=C$ to $k=C+1$, the Manhattan distance increases by $\abs{P_{a}[C+1] - P_{b}[C+1]}$.
Second, note that edit distances are also additive. 
That is, by inserting a single bit into the same position in each of the two vectors,
the edit distance increases by the edit distance between the two inserted bits.
Therefore, there are four cases to consider (just like in the base case), and for each case,
edit distance increases by the same amount as the increase in Manhattan distance, thus, proving the induction.

\section{Original MDS Algorithm}

\begin{algorithm}[t]
{\footnotesize
\begin{algorithmic}
\Procedure{update-sample}{$x$}
	\State{$S[x]$.clear()}
	\For{$i \leftarrow 0, \: i < S[x].\text{capacity}() + N[x].\text{capacity}()$}
		\State{$y \leftarrow$ rand()$\%k$}
		\If{$N[x]$.isFull()}
			\If{$\delta^{H}(x, y) < \delta^{H}(x, N[x]$.peek()$)$}
				\State{$S[x]$.push($N[x]$.pop())}
				\State{$N[x]$.push($y$)}
			\Else
				\State{$S[x]$.push($y$)}
			\EndIf
		\Else
			\State{$N[x]$.push($y$)}
		\EndIf
		\State{$i\texttt{++}$}
	\EndFor
\EndProcedure
\Procedure{update-velocity}{$x$}
	\State{$f \leftarrow 0$}
	\ForAll{$y \in S[x] \cup N[x]$}
		\If{$X[x] < X[y]$}
			\State $f \mathrel{+}= \bigl\lvert X[x] - X[y] \bigr\rvert - \delta^{H}(x, y)$
		\Else
			\State $f \mathrel{+}= \delta^{H}(x, y) - \bigl\lvert X[x] - X[y] \bigr\rvert$ 
		\EndIf
	\EndFor
	\State{$f \leftarrow f / \bigl\lvert S[x] \cup N[x] \bigr\rvert$}
	\State{$V[x] \leftarrow V[x] / 2 + f$}
\EndProcedure
\Procedure{update-coordinates}{$x$}
	\State{$X[x] \mathrel{+}= V[x]$}
\EndProcedure
\end{algorithmic}
}
\caption{}
\label{alg:original}
\end{algorithm}

For completeness, first, we summarize the steps in the original MDS algorithm~\cite{} and subsequently, describe our specific adaptations.
The major building blocks of the algorithm are depicted in Algorithm~\ref{alg:original}.
The algorithm is based on a spring-force analogy.
Initially, MDS points are (uniformly) randomly scattered in the coordinate space, but in successive iterations the algorithm re-positions these points.
For every pair of points, it is assumed that the points exert a (positive/negative) force on each other 
proportional to the difference between their original distances and their distances in the coordinate space.
In every iteration, using laws of classical physics,
for any given pair of points, their acceleration can be computed/updated, which, in turn, can be used for 
updating the velocities (cf., \textsc{update-velocities} in Algorithm~\ref{alg:original}) and 
coordinates (cf., \textsc{update-coordinates} in Algorithm~\ref{alg:original}) of the points.
Since computing the force between every pair of points is not scalable, 
the authors propose an approximation in which forces are computed with respect to only a subset of points.
In each iteration, the algorithm takes additional steps to ensure that this sample becomes increasingly more representative of the true population (cf., \textsc{update-sample} in Algorithm~\ref{alg:original}).
Consequently, the points are iteratively re-positioned until the forces converge or in the worst case, for a predefined number of iterations.
